# Supplementary material for: Extreme Model Compression for On-device Natural Language Understanding
Source: arXiv:2012.00124 source file (2020-11-30)
Supplement: Supplementary file 1 [file appendix.tex]

\section{Memory Profile for models}
Word Embedding Layers: 69MB\\BiLSTM Layers: 9.5MB\\
Classification and tagging layers: 0.94MB

\section{Data Relabeling Strategies} \label{app:data_label}
In order to train models suitable for on-device NLU, we prepare different datasets to assist in training, evaluation and testing of candidate models. We start with the same dataset that cloud uses for training its models. This is a curated list of annotated utterances that were either mined and annotated from the live production traffic or are generated synthetically (using rules and grammars). An utterance annotation in this dataset contains its domain label, intent label and the slot labels for all the words in the utterance. However, since the on-device NLU supports only a subset of cloud domains and intents, we apply multiple re-labeling strategies to the utterance annotations. These re-labeling strategies revolve around the basic idea of how we treat annotated labels for utterances that belong to non-supported domain or intent. 

\section{Dataset Selection Experiments} \label{app:data_sel}
The model configuration used for this stage is: Bi-LSTM Hidden Size: \textbf{512}; Tagging Architecture: \textbf{CRF}; Number of Bi-LSTM layers: \textbf{1}; Pre-trained Embeddings: \textbf{Alexa300}. 

\section{SVD Based Compression - Analysis}
 \begin{figure}[tb]
 	\centering
 	\includegraphics[width=0.8\linewidth]{singular_val_vs_component_100_dim.png}
 	\caption{Singular Values vs \# SVD components retained}
 	\label{fig:svd1}
 \end{figure}
 
  \begin{figure}[tb]
 	\centering
 	\includegraphics[width=0.8\linewidth]{SVD_reconstruction_loss_vs_num_components_100.png}
 	\caption{SVD Reconstruction loss vs \# SVD components retained}
 	\label{fig:svd2}
 \end{figure}
 
  \begin{figure}[tb]
 	\centering
 	\includegraphics[width=0.8\linewidth]{irer_vs_svd.png}
 	\caption{IRER vs \# SVD components retained}
 	\label{fig:svd3}
 \end{figure}
